# Supplementary material for: A Conceptual Framework for Human-AI Collaborative Genome Annotation
Source: arXiv:2503.23691 source file (2025-03-31)
Supplement: Supplementary file 1 [file suppl.pdf]

# Supplementary Notes of 'A Conceptual Framework for Human-AI Collaborative Genome Annotation'

## Supplementary Note 1: Automated genome annotation

### Evolution of automated genome annotation

Automated genome annotation usually consists of several steps, including sequence alignment, masking repeat sequences, identifying genomic elements, predicting their functions, and performing quality control (McEntyre and Ostell, 2002). Numerous computational methods have been developed for each step of the genome annotation process. A rough chronology can be outlined based on the emergence and prominence of various methods.

In the 1990s and 2000s, rule-based and heuristic methods were the most common approaches for genome annotation. These methods relied on predefined rules or heuristics to identify genes in genome sequences. Tools like BLAST (Altschul et al., 1990) became essential for similarity-based annotations, while gene prediction software such as Glimmer (Delcher et al., 1999) for prokaryotes and AUGUSTUS (Stanke et al., 2003) for eukaryotes utilized statistical models like hidden Markov models (HMMs). These methods are commonly referred to as homology-based (e.g., BLAST) and *ab initio* (e.g., Glimmer and AUGUSTUS) approaches in the literature. Homology-based methods compare the target genome sequence to a database of known genes, which serve as templates. If the target sequence is similar to a known gene, it is likely that the sequence also encodes a gene with similar functions. *Ab initio* methods, on the other hand, detect protein-coding genes by identifying conserved features within the target genome. These conserved features include statistical properties of protein-coding sequences and regulatory signals surrounding protein-coding genes (Tiwari et al., 1997).

In the 2000s and 2010s, integrated and ensemble methods became increasingly popular. These approaches combined multiple sources of evidence to improve prediction accuracy. Tools like MAKER (Holt and Yandell, 2011) integrated *ab initio* gene predictions, protein homology, and transcript evidence. Meanwhile, ensemble methods such as EVidenceModeler (Haas et al., 2008) combined outputs from multiple annotation tools to derive consensus annotations.

In the 2010s and 2020s, ML and deep learning methods have been used to improve the accuracy of genome annotation. Traditional ML techniques, including support vector machines (SVMs) and random forest (RFs), began to be used for various tasks in GA (Mahood et al., 2020). Deep learning methods, such as convolutional neural networks

(CNNs), have been employed for predicting gene structures, regulatory elements, and other genomic features (Mahood et al., 2020; Sapoval et al., 2022; Zou et al., 2019). Well-known examples include AlphaFold3 (Abramson et al., 2024) for biomolecular structure prediction and SpliceAI (Jaganathan et al., 2019) for splice site prediction.

The 2020s have marked a revolutionary era in genome annotation with the rise of Generative AI and advanced machine learning technologies. One prominent example is AlphaFold3 (Abramson et al., 2024), which continues to redefine biomolecular structure prediction with unprecedented accuracy and scalability. Generative AI has further expanded its capabilities with diffusion models that can design proteins with desired properties (Watson et al., 2023). These advancements have significant implications for understanding complex biological processes and engineering novel biomolecules. Large Language Models (LLMs), such as ChatGPT, have gained global attention for their ability to process and generate human language. Their applications extend beyond language processing to the analysis of sequential biological data, including DNA, proteins, and gene expression. In the life sciences, LLMs have been trained on diverse datasets encompassing natural language, molecular sequences, protein structures, and genomic information (Zhang et al., 2024).

New methods are constantly being developed, and existing methods are continually refined in response to growing datasets, our ever-expanding understanding of genomics, and emerging biotechnologies. For example, long-read sequencing techniques, such as those offered by Pacific Biosciences (PacBio) and Oxford Nanopore Technologies (ONT), have dramatically improved genome assembly (Logsdon et al., 2020). New computational methods are required to process long-read sequencing data (Amarasinghe et al., 2020) or integrate short- and long-read sequencing data (Olson et al., 2022).

## Automated genome annotation pipeline

In practice, genome annotation is performed using a genome annotation pipeline, which consists of a series of computational tools. One or more specialized computational tools are employed at each step of the process. These multiple computationally intensive steps are executed in a predefined order, handling various data sources such as aligned sequences, RNA-seq data, and protein information (Holt and Yandell, 2011; McEntyre and Ostell, 2002; Fiddes et al., 2018; Banerjee et al., 2021; Solovyev et al., 2006). Many biological analyses rely on pipelines that have been established and validated over many years. The adoption of new methodologies requires rigorous validation to ensure that new pipelines are both accessible and reliable. While deep learning and advanced AI techniques have seen significant advances and applications in many fields, their full-scale adoption in genome annotation may still be ahead of us.

## Challenges in automated genome annotation

### Lack of gold-standard data

Since computational tools, particularly ML/AI models, learn from data, the quality of input data directly affects the effectiveness and reliability of the resulting models. However, genome databases, especially those for non-model species, often contain incomplete or inaccurate data. Even in well-studied model species such as Arabidopsis thaliana, a substantial proportion of genes (36%) still lack molecular function or biological process

annotations (TAIR database, as of July 2016) (Bolger et al., 2018). The challenge is even greater for non-model species, where annotations are primarily inferred from model organisms without species-specific experimental validation.

Additionally, public genome databases have been found to contain substantial errors (Bolger et al., 2018; Schnoes et al., 2009). Errors can arise at various stages of genome analysis (Bolger et al., 2018; Müller et al., 2003). One of the primary causes of annotation errors is contamination within assemblies, which has been detected in nearly all major databases (Bensch et al., 2021; Bolger et al., 2018). These errors propagate through downstream analyses (Kyrpides, 2009) and are amplified by other ML/AI models (Hall et al., 2022). This creates a feedback loop in which low-quality data not only compromise current annotations but also undermine future studies that rely on these databases.

### Generalizing a model to a new species

The scarcity of diverse datasets significantly hampers a models' ability to generalize and perform effectively across a wide range of genomic contexts. This limitation not only restricts models' training but also undermines their capacity to discover novel patterns and make accurate predictions in less-studied species.

For example, homology-based models transfer the annotations of homologous genes to target genes based on sequence or structural similarity (Korf et al., 2001; Keilwagen et al., 2016; van Baren and Brent, 2006). However, these models struggle to recognize novel genomic elements that lack homologous sequences in existing databases, such as species-specific genes and newly sequenced genomes with long evolutionary distances from reference genomes. The performance of homologous gene annotation depends on the completeness and quality of genome assemblies and the accuracy of reference genome annotations.

*Ab initio* models are often trained on a specific species (Lomsadze et al., 2005; Burge and Karlin, 1997; Salamov and Solovyev, 2000). They optimize performance by leveraging available signals in the training data, which may be specific to that dataset. As a result, their ability to generalize to new species is impaired.

### Integrating multi-omics data.

An increasing number of innovative approaches, including integrated methods (Holt and Yandell, 2011) and hybrid methods (Bruna et al., 2020; Stanke et al., 2006; Solovyev et al., 2006), combine multiple omics data to achieve more accurate and comprehensive genome annotation. However, these methods are often limited by incomplete evidence or insufficient training data, particularly in non-model species, where the quantity and quality of available data for each omic may vary. Additionally, integrating multi-omics data into ML/AI models remains challenging due to the high-dimensional and heterogeneous nature of such data (Barua et al., 2023).

### Interpreting ML/AI models.

ML/AI, particularly deep learning algorithms, have recently garnered increasing interest in various genome annotation tasks (Eraslan et al., 2019; Zou et al., 2019). Deep learning methods can significantly improve genome annotation accuracy (Abramson et al., 2024), but their results are more challenging to interpret than those of traditional ML/AI approaches (Talukder et al., 2021). This complexity obscures the understanding of deep

learning models' predictive mechanisms and makes pinpointing potential inaccuracies in the annotation process more difficult.

# Supplementary Note 2: Manual curation

## Overview of manual curation

Manual genome curation can be categorized into three primary approaches: *museum*, *cottage industry* and *jamboree* (Stein, 2001). The museum approach relies on a centralized team of experts responsible for curating the entire genome, usually for well-studied model species. In the cottage industry approach, multiple independent curators contribute to different regions of the genome. The jamboree approach brings together a large group of participants to collaborate on a genome annotation project. While this approach can expedite the process and reduce costs, it requires robust quality control mechanisms to ensure consistency. Community-based curation (Rödelsperger et al., 2019) and crowd-sourcing biocuration (Ramsey et al., 2021) are examples of the jamboree approach.

The manual curation process may vary depending on the specific project. However, some common steps can be followed in manual curation, as shown in Figure 1.

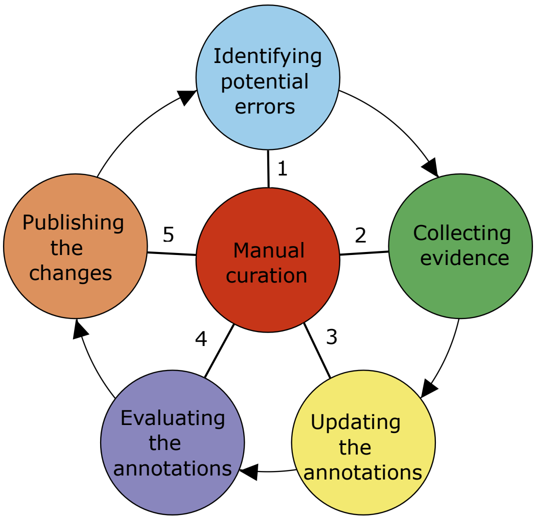


Figure 1: Overview of manual curation.

**Step 1**: Identifying potential errors in genome annotation Potential errors may occur in features such as assembly gap regions, non-canonical splice sites, multiple alternative splicing forms, trans-spliced genes, and putative gene functions lacking sufficient evidence. Curators can compare genome annotations against external evidence to detect regions that deviate from the expected structure or function of known genes. They can also identify discrepancies where predicted gene models are annotated differently by various pipelines (McDonnell et al., 2018).

**Step 2**: Collecting evidence to enhance genome annotation To improve the understanding of genomic elements, curators can gather diverse lines of evidence. For instance, experimental data, such as RNA and protein sequences, are useful for confirming the presence or absence of transcripts and determining the exon-intron structure of genes (Cheng et al., 2017). Furthermore, public databases such as GenBank (Sayers et al.,

2020), RefSeq (O'Leary et al., 2016), UniProt (The UniProt Consortium, 2023), InterPro (Paysan-Lafosse et al., 2023), Pfam (Mistry et al., 2021), GO (Gene Ontology Consortium, 2021), and KEGG (Kanehisa and Goto, 2000) provide invaluable information on nucleotide and protein sequences, as well as various functional annotations. Finally, extensive research literature can offer additional experimental gene annotations and sequences that may not be available in public databases.

**Step 3**: Updating the annotations based on evidence Once evidence is collected, curators can update genome annotations accordingly. For example, gene boundaries can be refined by reviewing RNA or protein sequence alignments. Multiple alternative splicing forms can be identified using RNA-Seq data from various conditions and tissues. Untranslated regions (UTRs) missing from automated GA can be recovered using short peptide data (Madupu et al., 2010). Pseudogenes can be detected by identifying incomplete protein domains in predicted gene models (McDonnell et al., 2018). Such manual curation helps reduce error rates in genome annotation.

**Step 4**: Evaluating the updated annotations To ensure annotation accuracy, curators should identify any inconsistencies (McDonnell et al., 2018). For example, they can search for homologous genes and assess their functional relationships. Genes with high similarity, belonging to the same gene families or a particular group, should be assigned the same functional annotation. While not an absolute rule, this guideline helps curators maintain consistency in annotations.

**Step 5**: Publishing the updated annotations and corresponding evidence to public databases Publishing updated annotations in public databases is crucial for enriching scientific knowledge and advancing research (Ramsey et al., 2021). While large-scale projects typically share their updated annotations, smaller projects may focus on identifying genes of interest without immediately submitting their changes to public databases.

## Support tools and systems

Online platforms such as GeneDB (Manske et al., 2019) and other Wiki-based systems (listed at https://ngdc.cncb.ac.cn/sciencewikis/index.php/Biological_Wikis) allow registered users to collaboratively create and edit genome annotation pages in real time (Ramsey et al., 2021). This approach decentralizes the curation process and leverages the collective expertise of the global community. However, a key concern with Wiki-based systems is that open editing may introduce errors and biases.

In contrast, standalone and web-based curation systems can be used within more defined teams and projects. For example, the AceDB annotation editor and its variants have been used for C. elegans, the human genome sequence, and the Berkeley Drosophila Genome Project (Consortium, 1999; Frankish and Harrow, 2014). Artemis and the Artemis Comparison Tool (ACT) were primarily designed for reviewing smaller prokaryotic or eukaryotic genomes (Rutherford et al., 2000) but have since been extended to more complex genomes (Carver et al., 2008, 2012). Neomorphic's Annotation Station gene editor was used in The Institute for Genomic Research (TIGR) program for the re-annotation of the Arabidopsis genome (Haas et al., 2005). yrGATE has been used to correct exon-intron structures of genes in several plant-specific databases (Wilkerson et al., 2006). Manual Annotation Studio (MAS) was developed to improve the efficiency of manual functional annotation of prokaryotic and viral genomes (Lueder et al., 2021). DNA Master has

been used for bacteriophage genome annotation (Salisbury and Tsourkas, 2019). MaGe has been used to refine the automatic prediction of gene product functions in bacterial genomes (Vallenet et al., 2006). PeerGAD was a peer-review-based, community-centric web application for viewing and annotating prokaryotic genome sequences (D'Ascenzo et al., 2004). Manatee, developed by The Institute for Genomic Research (TIGR), has been widely used for microbial genome annotation (Haas et al., 2005).

Recently, Apollo has gained widespread adoption within the genome annotation (GA) community (Dunn et al., 2019). Many GA projects integrate this editing tool and use it to annotate various genomes, including GadFly (Mungall et al., 2002), Galaxy (Ramsey et al., 2020) (e.g., G-OnRamp (Liu et al., 2019)), GeneSAS (Humann et al., 2019), DNA Subway (Hilgert et al., 2014), Bovine [Childers et al. (2011); triant2020using], VectorBase (Giraldo-Calderón et al., 2022), VEuPathDB (Amos et al., 2022), and the i5k workspace (Poelchau et al., 2015). Apollo also plays a crucial role in community-driven GA projects, such as the "Genome Decoders" initiative by the Sanger Institute and WormBase, where school students collaborate to annotate the human whipworm genome (Dunn et al., 2019).

These systems provide a platform for aggregating information from diverse databases and curators. While they integrate multiple tools designed for specific tasks, they may still require external tools to support additional functions, particularly for curating information from scientific literature. Scientific literature is invaluable for identifying genes extensively studied in wet-lab experiments, where gene labels are considered the gold standard for gene functions.

Text mining tools have been employed to accelerate two key processes in manual curation: literature searching and information retrieval (Drabkin et al., 2012).

Literature searching tools, such as Textpresso (Müller et al., 2018) and PubSearch (Yoo et al., 2006), identify the most relevant publications related to genes of interest. Users can search the literature using keywords, including gene names, article metadata, and ontology terms. These tools generate indexes that link keywords to articles, enabling curators to efficiently review target genes and their associated publications.

Information retrieval tools extract key concepts for users to review, such as PubTator (Wei et al., 2019), NCBOAnnotator (Tchechmedjiev et al., 2018), Canto (Rutherford et al., 2014), and OntoMate (Liu et al., 2015). Additionally, various natural language processing (NLP) methods can be incorporated into these systems for biological entity recognition, entity linking, and relation extraction (Luo et al., 2023; Lee et al., 2020; Li et al., 2019; Fang et al., 2023). For example, biological entity recognition extracts gene names, mutations, and species from the text; entity linking connects these entities to their corresponding entries in a knowledge base or ontology; and relation extraction identifies relationships between entities, such as gene-disease associations, which are crucial for knowledge discovery.

# Supplementary Note 3: Humans collaborate with AI systems

**Learning.** Human curators engage in domain learning in genomics to make accurate annotation judgement. Additionally, through experience on a task, humans build "mental

models", mental representations of the key elements of a task (e.g.~theoretical concepts, task steps and actors) and how these components interact (Cannon-Bowers et al., 1993). This includes an understanding of their teammates and how the team works together to achieve the goal. In the HAICoGA context, humans learn from their experiences working with AI to help understand the strengths and limitations of AI and themselves (Andrews et al., 2022).

**Reasoning.** Human reasoning is characterized by creativity, intuition, and the ability to deal with unstructured information through experience and learning. (Patterson, 2017, zheng2017hybrid). Unlike AI systems, human reasoning excels in abstract thinking and dynamic problem-solving. This ability stems from the human brain's intricate neural structure, enabling the integration of past experiences, contextual understanding, and intuitive judgment. Humans can synthesize disparate pieces of information, make decisions in uncertain conditions, and adapt to new situations swiftly, showcasing a level of flexibility and depth that current AI systems struggle to replicate. This inherent complexity and adaptability make human reasoning an invaluable component in collaborative human-AI systems (Zheng et al., 2017).

**Situational awareness.** Human situational awareness, as it is commonly defined, refers to an agent's (1) perception of the key information or elements in the task, (2) comprehension of their meaning and (3) predictions about how the situation will unfold (Endsley, 1995). Situational awareness develops dynamically during a task as humans engage in "sense-making" (Klein et al., 2006), and it plays a critical role in task performance (Endsley, 1995). When working with AI, situational awareness includes the ability to monitor the actions of AI and execute corresponding responses, which can increase the effectiveness of collaborations (Jiang et al., 2022). For example, humans will know how best to put prompts to a chatbot by investigating information in conversations (Lou et al., 2023).

**Decision** Humans make decisions based on their judgment, situation, knowledge or a combination of available data. Considering functional annotations of genes by GO, all annotations need to be supported with statements of evidence and source publications (McDonnell et al., 2018). Human curators need to decide the GO term and evidence code for each annotation using their expertise and a variety of data from the peer-reviewed literature. Humans utilize their judgment in decision-making to navigate complex situations. For example, even with curator expertise and supporting evidence, full certainty cannot be achieved. Curators' judgments lead them to make decisions under some uncertainty (with lower confidence) or postpone decision-making until new evidence is available. Moreover, whether to accept an AI's suggestion is often left to individual curators' judgments and is likely not very standardized. While there are default parameter settings in specific databases or models, the exact thresholds used in methods can vary based on the research question, the dataset, and the researcher's judgment.

**Delegation.** Humans can delegate tasks to leverage complementary AI competencies(Pinski et al., 2023). Deciding to delegate to AI is based on, among other things, the human's assessment of the AI's ability and confidence in their own (Fügener et al., 2019). Due to the speed, scalability and quantitative capabilities of AI, humans usually make AI automatically annotate a large scale of the genome, or require AI to provide relevant information about gene annotations by searching databases and literature.

**Trust.** Ensuring appropriate levels of trust is particularly important to establish success-

ful collaborative relationships between humans and AI. Ideally, the human-AI system should support "calibrated" trust that aligns accurately with the AI's capabilities (Lee and See, 2004). In long-term collaborations, this calibrated trust becomes even more critical, as it ensures a balanced reliance on AI over time. Trust should be neither too low, causing humans to disengage from the AI, nor too high, leading to overreliance and potential failure to detect errors. Maintaining this balance is essential for sustained collaboration, where the dynamics of trust evolve with ongoing interactions and experiences.

# Supplementary Note 4: AI systems collaborate with humans

**Learning.** AI systems are designed to learn from data and develop their ability to perform tasks using various strategies, such as supervised (Scalzitti et al., 2020), semi-supervised (Jia et al., 2021), and unsupervised learning (Abeel et al., 2008), all of which have already been applied in genome annotation. In HAICoGA, we may leverage additional AI learning strategies, such as reinforcement learning, continuous learning, and active learning, to enhance AI-human collaboration.

Reinforcement learning is a valuable strategy for enhancing human-AI collaboration by enabling AI to learn from and work alongside humans (Navidi and Landry Jr, 2021). It can help AI make decisions and take actions aligned with team goals, adapt to the environment, and improve overall team performance.

Continuous learning refers to an AI system's ability to learn from new data streams in real time without requiring complete retraining (Wang et al., 2022). This capability is crucial for human-AI collaboration, particularly in dynamic environments where conditions and information constantly evolve. Through continuous learning, AI can adapt to new scenarios, update its knowledge, and refine its decision-making processes in response to changing inputs. This flexibility ensures that AI remains relevant and effective over time, enhancing its ability to support humans.

Active learning involves the strategic selection of data samples for human labeling to maximize information gain while minimizing human effort (van der Wal et al., 2021). A potential use case is AI identifying genomic regions with high uncertainty but significant relevance to GA. Humans can then focus their efforts on these informative regions rather than the entire genome.

**Co-learning.** Co-learning refers to the process in which humans and AI learn from each other through collaborative interactions (van den Bosch et al., 2019). The benefits of human-AI co-learning have been demonstrated in various studies. For example, one study proposed that co-learning fosters mutual understanding, mutual benefits, and mutual growth between humans and AI, ultimately enhancing productivity and creativity (Huang et al., 2019). Another study suggested that co-learning enables humans and AI to discover and understand the task, environment, themselves, and their teammates (Schoonderwoerd et al., 2022). Several methods have been developed to facilitate AI co-learning with humans and achieve optimal performance by integrating various learning strategies [Mozannar and Sontag (2020); van2021biological].

**Reasoning.** AI reasoning usually excels in logicality, repeatability, and the efficient

processing of structured data through predefined rules and machine learning algorithms (Zheng et al., 2017). This enables AI systems to handle large volumes of data and perform complex calculations at speeds unattainable by humans. However, in the context of human-AI collaboration, improving AI reasoning requires integrating human-like cognitive elements, such as intuitive reasoning and contextual understanding (Zheng et al., 2017). Enhancing AI reasoning involves developing systems capable of learning from diverse, dynamic, and unstructured environments. Another critical aspect of improving AI reasoning is the development of causal models, which allow AI to understand and predict relationships between variables beyond mere correlations (Shipley, 2016; Hill et al., 2016). Causal reasoning helps AI interpret cause-effect relationships, making decision-making processes more transparent and explainable (Zheng et al., 2017).

**Situational awareness.** AI's situational awareness refers to its ability to detect, analyze, and respond to environmental changes while taking appropriate actions based on that information (Jiang et al., 2022). Traditionally, human situational awareness is assessed through working memory and verbalization skills (Berglund et al., 2023). In AI systems, situational awareness is achieved through a combination of perception (Gathering data from the environment), comprehension (Interpreting the data and understanding the context), and projection (Predicting future states of the environment based on current information) mechanisms (Munir et al., 2022).

**Shared situational awareness.** Shared situational awareness refers to the extent to which both humans and AI have a mutual understanding of environmental changes. It emphasizes the importance of real-time information sharing and transparent communication between humans and AI (Andrews et al., 2022).

**Prediction.** In the context of HAICoGA, AI systems play a critical role in predicting gene structures and functions, while human experts review and refine these predictions to ensure they align with existing evidence and domain knowledge. As AI systems improve in accuracy and reliability, they are expected to contribute more significantly to decision-making processes. Beyond generating raw predictions, AI in human-AI collaboration should develop contextual understanding and anticipate the next steps or interactions required. For example, AI might predict necessary adjustments or identify areas requiring further investigation, thereby dynamically guiding the collaboration. While prediction is a key function, AI also supports tasks such as clustering and information retrieval, each enhancing different aspects of genome annotation. Tools like quality metrics and gene tree visualizers illustrate this by helping to identify misannotations that require human correction (Tello-Ruiz et al., 2019).

**Delegation.** AI systems are expected to delegate certain tasks to humans rather than risk generating incorrect annotations. For example, AI could assign difficult genes, such as very short genes, pseudogenes, or tandem gene duplications, to human experts when it struggles with them (Madupu et al., 2010). In the current manual curation process, genes lacking GO annotations, those with non-canonical splice sites, or poorly annotated genes are delegated to human curators (Tello-Ruiz et al., 2019). Such methods can be considered one-off delegation strategies. With advanced AI methods (Mozannar and Sontag, 2020), we can also design intrinsic delegation strategies, allowing AI systems to dynamically delegate tasks to humans in long-term collaborations.

**Explainability.** The explainability of AI refers to its ability to provide a human-

understandable rationale for its results. "White-box" models, such as those based on patterns, rules, or decision trees, explicitly explain how they generate predictions and have been widely used in biomedical research. However, "black-box" models, particularly deep learning models, outperform white-box models in complex tasks but lack the transparency needed to produce explainable knowledge (Dey et al., 2022). This can pose challenges in understanding biological mechanisms and building trust in AI-generated conclusions (Ali et al., 2023). These challenges are being addressed through explainable artificial intelligence (XAI) techniques, which enhance the interpretability of black-box models. Such advancements boost confidence in AI-generated outputs across a wide range of biological applications (Zhou et al., 2023; Koh et al., 2024).

# References


Abeel, Thomas, Yvan Saeys, Pierre Rouzé, and Yves Van de Peer (2008), "ProSOM: core promoter prediction based on unsupervised clustering of DNA physical profiles." *Bioinformatics*, 24, i24.

Abramson, Josh, Jonas Adler, Jack Dunger, Richard Evans, Tim Green, Alexander Pritzel, Olaf Ronneberger, Lindsay Willmore, Andrew J Ballard, Joshua Bambrick, et al. (2024), "Accurate structure prediction of biomolecular interactions with alphafold 3." *Nature*, 1–3.

Ali, Sajid, Tamer Abuhmed, Shaker El-Sappagh, Khan Muhammad, Jose M Alonso-Moral, Roberto Confalonieri, Riccardo Guidotti, Javier Del Ser, Natalia Díaz-Rodríguez, and Francisco Herrera (2023), "Explainable artificial intelligence (xai): What we know and what is left to attain trustworthy artificial intelligence." *Information fusion*, 99, 101805.

Altschul, Stephen F, Warren Gish, Webb Miller, Eugene W Myers, and David J Lipman (1990), "Basic local alignment search tool." *Journal of molecular biology*, 215, 403–410.

Amarasinghe, Shanika L, Shian Su, Xueyi Dong, Luke Zappia, Matthew E Ritchie, and Quentin Gouil (2020), "Opportunities and challenges in long-read sequencing data analysis." *Genome biology*, 21, 1–16.

Amos, Beatrice, Cristina Aurrecoechea, Matthieu Barba, Ana Barreto, Evelina Y Basenko, Robert Belnap, Ann S Blevins, Ulrike Böhme, John Brestelli, Brian P Brunk, et al. (2022), "Veupathdb: the eukaryotic pathogen, vector and host bioinformatics resource center." *Nucleic Acids Research*, 50, D898–D911.

Andrews, Robert W, J Mason Lilly, Divya Srivastava, and Karen M Feigh (2022), "The role of shared mental models in human-ai teams: a theoretical review." *Theoretical Issues in Ergonomics Science*, 1–47.

Banerjee, Sagnik, Priyanka Bhandary, Margaret Woodhouse, Taner Z Sen, Roger P Wise, and Carson M Andorf (2021), "Finder: an automated software package to annotate eukaryotic genes from rna-seq data and associated protein sequences." *BMC bioinformatics*, 22, 1–26.

Barua, Arnab, Mobyen Uddin Ahmed, and Shahina Begum (2023), "A systematic literature review on multimodal machine learning: Applications, challenges, gaps and future directions." *IEEE Access*, 11, 14804–14831.

Bensch, Staffan, Mizue Inumaru, Yukita Sato, Larisa Lee Cruz, Andrew A Cunningham, Simon J Goodman, Iris I Levin, Patricia G Parker, Patricia Casanueva, Maria-Angeles Hernández, et al. (2021), "Contaminations contaminate common databases." *Molecular ecology resources*, 21, 355–362.

Berglund, Lukas, Asa Cooper Stickland, Mikita Balesni, Max Kaufmann, Meg Tong, Tomasz Korbak, Daniel Kokotajlo, and Owain Evans (2023), "Taken out of context: On measuring situational awareness in llms." *arXiv preprint arXiv:2309.00667*.

Bolger, Marie E, Borjana Arsova, and Björn Usadel (2018), "Plant genome and transcriptome annotations: from misconceptions to simple solutions." *Briefings in bioinformatics*, 19, 437–449.

Bruna, Tomáš, Alexandre Lomsadze, and Mark Borodovsky (2020), "Genemark-ep+: eukaryotic gene prediction with self-training in the space of genes and proteins." *NAR genomics and bioinformatics*, 2, lqaa026.

Burge, Chris and Samuel Karlin (1997), "Prediction of complete gene structures in human genomic dna." *Journal of molecular biology*, 268, 78–94.

Cannon-Bowers, Janis A, Eduardo Salas, and Sharolyn Converse (1993), "Shared mental models in expert team decision making." *Individual and group decision making: Current issues*, 221–246.

Carver, Tim, Matthew Berriman, Adrian Tivey, Chinmay Patel, Ulrike Böhme, Barclay G Barrell, Julian Parkhill, and Marie-Adèle Rajandream (2008), "Artemis and act: viewing, annotating and comparing sequences stored in a relational database." *Bioinformatics*, 24, 2672–2676.

Carver, Tim, Simon R Harris, Matthew Berriman, Julian Parkhill, and Jacqueline A McQuillan (2012), "Artemis: an integrated platform for visualization and analysis of high-throughput sequence-based experimental data." *Bioinformatics*, 28, 464–469.

Cheng, Chia-Yi, Vivek Krishnakumar, Agnes P Chan, Françoise Thibaud-Nissen, Seth Schobel, and Christopher D Town (2017), "Araport11: a complete reannotation of the arabidopsis thaliana reference genome." *The Plant Journal*, 89, 789–804.

Childers, Christopher P, Justin T Reese, Jaideep P Sundaram, Donald C Vile, C Michael Dickens, Kevin L Childs, Hanni Salih, Anna K Bennett, Darren E Hagen, David L Adelson, et al. (2011), "Bovine genome database: integrated tools for genome annotation and discovery." *Nucleic acids research*, 39, D830–D834.

Consortium, FlyBase (1999), "The flybase database of the drosophila genome projects and community literature." *Nucleic Acids Research*, 27, 85–88.

Delcher, Arthur L, Douglas Harmon, Simon Kasif, Owen White, and Steven L Salzberg (1999), "Improved microbial gene identification with glimmer." *Nucleic acids research*, 27, 4636–4641.

Dey, Sanjoy, Prithwish Chakraborty, Bum Chul Kwon, Amit Dhurandhar, Mohamed Ghalwash, Fernando J Suarez Saiz, Kenney Ng, Daby Sow, Kush R Varshney, and Pablo Meyer (2022), "Human-centered explainability for life sciences, healthcare, and medical informatics." *Patterns*, 3, 100493.

Drabkin, Harold J, Judith A Blake, and Mouse Genome Informatics Database (2012), "Manual gene ontology annotation workflow at the mouse genome informatics database." *Database*, 2012, bas045.

Dunn, Nathan A, Deepak R Unni, Colin Diesh, Monica Munoz-Torres, Nomi L Harris, Eric Yao, Helena Rasche, Ian H Holmes, Christine G Elsik, and Suzanna E Lewis (2019), "Apollo: democratizing genome annotation." *PLoS computational biology*, 15, e1006790.

D'Ascenzo, Mark D, Alan Collmer, and Gregory B Martin (2004), "Peergad: a peer-review-based and community-centric web application for viewing and annotating prokaryotic genome sequences." *Nucleic acids research*, 32, 3124–3135.

Endsley, Mica R (1995), "Toward a theory of situation awareness in dynamic systems." *Human factors*, 37, 32–64.

Eraslan, Gökcen, Žiga Avsec, Julien Gagneur, and Fabian J Theis (2019), "Deep learning: new computational modelling techniques for genomics." *Nature Reviews Genetics*, 20, 389–403.

Fang, Li, Qingyu Chen, Chih-Hsuan Wei, Zhiyong Lu, and Kai Wang (2023), "Bioformer: an efficient transformer language model for biomedical text mining." *arXiv preprint arXiv:2302.01588*.

Fiddes, Ian T, Joel Armstrong, Mark Diekhans, Stefanie Nachtweide, Zev N Kronenberg, Jason G Underwood, David Gordon, Dent Earl, Thomas Keane, Evan E Eichler, et al. (2018), "Comparative annotation toolkit (cat)—simultaneous clade and personal genome annotation." *Genome research*, 28, 1029–1038.

Frankish, Adam and Jennifer Harrow (2014), "Gencode pseudogenes." In *Pseudogenes*, 129–155, Springer.

Fügener, Andreas, Jörn Grahl, Alok Gupta, and Wolfgang Ketter (2019), "Cognitive challenges in human-ai collaboration: Investigating the path towards productive delegation." *Forthcoming, Information Systems Research*, 1–39.

Gene Ontology Consortium (2021), "The gene ontology resource: enriching a gold mine." *Nucleic acids research*, 49, D325–D334.

Giraldo-Calderón, Gloria I, Omar S Harb, Sarah A Kelly, Samuel SC Rund, David S Roos, and Mary Ann McDowell (2022), "Vectorbase. org updates: bioinformatic resources for invertebrate vectors of human pathogens and related organisms." *Current opinion in insect science*, 50, 100860.

Haas, Brian J, Steven L Salzberg, Wei Zhu, Mihaela Pertea, Jonathan E Allen, Joshua Orvis, Owen White, C Robin Buell, and Jennifer R Wortman (2008), "Automated eukaryotic gene structure annotation using evidencemodeler and the program to assemble spliced alignments." *Genome biology*, 9, 1–22.

Haas, Brian J, Jennifer R Wortman, Catherine M Ronning, Linda I Hannick, Roger K Smith, Rama Maiti, Agnes P Chan, Chunhui Yu, Maryam Farzad, Dongying Wu, et al. (2005), "Complete reannotation of the arabidopsis genome: methods, tools, protocols and the final release." *BMC biology*, 3, 1–19.

Hall, Melissa, Laurens van der Maaten, Laura Gustafson, and Aaron Adcock (2022), "A systematic study of bias amplification." *arXiv preprint arXiv:2201.11706*.

Hilgert, Uwe, Sheldon McKay, Mohammed Khalfan, Jason Williams, Cornel Ghiban, and David Micklos (2014), "Dna subway: making genome analysis egalitarian." In *Proceedings of the 2014 Annual Conference on Extreme Science and Engineering Discovery Environment*, 1–3.

Hill, Steven M, Laura M Heiser, Thomas Cokelaer, Michael Unger, Nicole K Nesser, Daniel E Carlin, Yang Zhang, Artem Sokolov, Evan O Paull, Chris K Wong, et al. (2016), "Inferring causal molecular networks: empirical assessment through a community-based effort." *Nature methods*, 13, 310–318.

Holt, Carson and Mark Yandell (2011), "Maker2: an annotation pipeline and genome-database management tool for second-generation genome projects." *BMC bioinformatics*, 12, 1–14.

Huang, Yi-Ching, Yu-Ting Cheng, Lin-Lin Chen, and Jane Yung-jen Hsu (2019), "Human-ai co-learning for data-driven ai." *arXiv preprint arXiv:1910.12544*.

Humann, Jodi L, Taein Lee, Stephen Ficklin, and Dorrie Main (2019), "Structural and functional annotation of eukaryotic genomes with gensas." In *Gene prediction*, 29–51, Springer.

Jaganathan, Kishore, Sofia Kyriazopoulou Panagiotopoulou, Jeremy F McRae, Siavash Fazel Darbandi, David Knowles, Yang I Li, Jack A Kosmicki, Juan Arbelaez, Wenwu Cui, Grace B Schwartz, et al. (2019), "Predicting splicing from primary sequence with deep learning." *Cell*, 176, 535–548.

Jia, Hao, Sung-Joon Park, and Kenta Nakai (2021), "A semi-supervised deep learning approach for predicting the functional effects of genomic non-coding variations." *BMC bioinformatics*, 22, 1–12.

Jiang, Jinglu, Alexander J Karran, Constantinos K Coursaris, Pierre-Majorique Léger, and Joerg Beringer (2022), "A situation awareness perspective on human-ai interaction: Tensions and opportunities." *International Journal of Human–Computer Interaction*, 1–18.

Kanehisa, Minoru and Susumu Goto (2000), "Kegg: kyoto encyclopedia of genes and genomes." *Nucleic acids research*, 28, 27–30.

Keilwagen, Jens, Michael Wenk, Jessica L Erickson, Martin H Schattat, Jan Grau, and Frank Hartung (2016), "Using intron position conservation for homology-based gene prediction." *Nucleic acids research*, 44, e89–e89.

Klein, Gary, Brian Moon, and Robert R Hoffman (2006), "Making sense of sensemaking 1: Alternative perspectives." *IEEE intelligent systems*, 21, 70–73.

Koh, Eugene, Rohan Shawn Sunil, Hilbert Yuen In Lam, and Marek Mutwil (2024), "Harnessing big data and artificial intelligence to study plant stress." *arXiv preprint arXiv:2404.15776*.

Korf, Ian, Paul Flicek, Daniel Duan, and Michael R Brent (2001), "Integrating genomic homology into gene structure prediction." *Bioinformatics*, 17, S140–S148.

Kyrpides, Nikos C (2009), "Fifteen years of microbial genomics: meeting the challenges and fulfilling the dream." *Nature biotechnology*, 27, 627–632.

Lee, Jinhyuk, Wonjin Yoon, Sungdong Kim, Donghyeon Kim, Sunkyu Kim, Chan Ho So, and Jaewoo Kang (2020), "Biobert: a pre-trained biomedical language representation model for biomedical text mining." *Bioinformatics*, 36, 1234–1240.

Lee, John D and Katrina A See (2004), "Trust in automation: Designing for appropriate reliance." *Human factors*, 46, 50–80.

Li, Xiaoya, Jingrong Feng, Yuxian Meng, Qinghong Han, Fei Wu, and Jiwei Li (2019), "A unified mrc framework for named entity recognition." *arXiv preprint arXiv:1910.11476.*

Liu, Weisong, Stanley JF Laulederkind, G Thomas Hayman, Shur-Jen Wang, Rajni Nigam, Jennifer R Smith, Jeff De Pons, Melinda R Dwinell, and Mary Shimoyama (2015), "Ontomate: a text-mining tool aiding curation at the rat genome database." *Database*, 2015, bau129.

Liu, Yating, Luke Sargent, Wilson Leung, Sarah CR Elgin, and Jeremy Goecks (2019), "G-onramp: a galaxy-based platform for collaborative annotation of eukaryotic genomes." *Bioinformatics*, 35, 4422–4423.

Logsdon, Glennis A, Mitchell R Vollger, and Evan E Eichler (2020), "Long-read human genome sequencing and its applications." *Nature Reviews Genetics*, 21, 597–614.

Lomsadze, Alexandre, Vardges Ter-Hovhannisyan, Yury O Chernoff, and Mark Borodovsky (2005), "Gene identification in novel eukaryotic genomes by self-training algorithm." *Nucleic acids research*, 33, 6494–6506.

Lou, Renze, Kai Zhang, and Wenpeng Yin (2023), "Is prompt all you need? no. a comprehensive and broader view of instruction learning." *arXiv preprint arXiv:2303.10475.*

Lueder, Matthew R, Regina Z Cer, Miles Patrick, Logan J Voegtly, Kyle A Long, Gregory K Rice, and Kimberly A Bishop-Lilly (2021), "Manual annotation studio (mas): A collaborative platform for manual functional annotation of viral and microbial genomes." *BMC genomics*, 22, 1–14.

Luo, Ling, Chih-Hsuan Wei, Po-Ting Lai, Robert Leaman, Qingyu Chen, and Zhiyong Lu (2023), "Aioner: all-in-one scheme-based biomedical named entity recognition using deep learning." *Bioinformatics*, 39, btad310.

Madupu, Ramana, Lauren M Brinkac, Jennifer Harrow, Laurens G Wilming, Ulrike Böhme, Philippe Lamesch, and Linda I Hannick (2010), "Meeting report: a workshop on best practices in genome annotation." *Database*, 2010, baq001.

Mahood, Elizabeth H, Lars H Kruse, and Gaurav D Moghe (2020), "Machine learning: a powerful tool for gene function prediction in plants." *Applications in Plant Sciences*, 8, e11376.

Manske, Magnus, Ulrike Böhme, Christoph Püthe, and Matt Berriman (2019), "Genedb and wikidata." *Wellcome open research*, 4, 114.

McDonnell, Erin, Kimchi Strasser, and Adrian Tsang (2018), "Manual gene curation and functional annotation." In *Fungal Genomics*, 185–208, Springer.

McEntyre, Jo and Jim Ostell (2002), "The ncbi handbook." *Bethesda (MD): National Center for Biotechnology Information (US).*

Mistry, Jaina, Sara Chuguransky, Lowri Williams, Matloob Qureshi, Gustavo A Salazar, Erik LL Sonnhammer, Silvio CE Tosatto, Lisanna Paladin, Shriya Raj, Lorna J Richardson, et al. (2021), "Pfam: The protein families database in 2021." *Nucleic acids research*, 49, D412–D419.

Mozannar, Hussein and David Sontag (2020), "Consistent estimators for learning to defer to an expert." In *International Conference on Machine Learning*, 7076–7087, PMLR.

Müller, H-M, Kimberly M Van Auken, Yuling Li, and Paul W Sternberg (2018), "Textpresso central: a customizable platform for searching, text mining, viewing, and curating biomedical literature." *BMC bioinformatics*, 19, 1–16.

Müller, Heiko, Felix Naumann, and Johann-Christoph Freytag (2003), "Data quality in genome databases." In *Proceedings of the Eighth International Conference on Information Quality.*

Mungall, CJ, S Misra, BP Berman, J Carlson, E Frise, N Harris, B Marshall, S Shu, JS Kaminker, SE Prochnik, et al. (2002), "An integrated computational pipeline and database to support whole-genome sequence annotation." *Genome Biology*, 3, 1–11.

Munir, Arslan, Alexander Aved, and Erik Blasch (2022), "Situational awareness: techniques, challenges, and prospects." *AI*, 3, 55–77.

Navidi, Neda and Rene Landry Jr (2021), "New approach in human-ai interaction by reinforcement-imitation learning." *Applied Sciences*, 11, 3068.

O'Leary, Nuala A, Mathew W Wright, J Rodney Brister, Stacy Ciufo, Diana Haddad, Rich McVeigh, Bhanu Rajput, Barbara Robbertse, Brian Smith-White, Danso Ako-Adjei, et al. (2016), "Reference sequence (refseq) database at ncbi: current status, taxonomic expansion, and functional annotation." *Nucleic acids research*, 44, D733–D745.

Olson, Nathan D, Justin Wagner, Jennifer McDaniel, Sarah H Stephens, Samuel T Westreich, Anish G Prasanna, Elaine Johanson, Emily Boja, Ezekiel J Maier, Omar Serang, et al. (2022), "Precisionfda truth challenge v2: Calling variants from short and long reads in difficult-to-map regions." *Cell Genomics*, 2, 100129.

Patterson, Robert Earl (2017), "Intuitive cognition and models of human–automation interaction." *Human factors*, 59, 101–115.

Paysan-Lafosse, Typhaine, Matthias Blum, Sara Chuguransky, Tiago Grego, Beatriz Lázaro Pinto, Gustavo A Salazar, Maxwell L Bileschi, Peer Bork, Alan Bridge, Lucy Colwell, et al. (2023), "Interpro in 2022." *Nucleic Acids Research*, 51, D418–D427.

Pinski, Marc, Martin Adam, and Alexander Benlian (2023), "Ai knowledge: Improving ai delegation through human enablement." In *Proceedings of the 2023 CHI Conference on Human Factors in Computing Systems*, 1–17.

Poelchau, Monica, Christopher Childers, Gary Moore, Vijaya Tsavatapalli, Jay Evans, Chien-Yueh Lee, Han Lin, Jun-Wei Lin, and Kevin Hackett (2015), "The i5k

workspace@ nal—enabling genomic data access, visualization and curation of arthropod genomes." *Nucleic acids research*, 43, D714–D719.

Ramsey, Jolene, Brenley McIntosh, Daniel Renfro, Suzanne A Aleksander, Sandra LaBonte, Curtis Ross, Adrienne E Zweifel, Nathan Liles, Shabnam Farrar, Jason J Gill, et al. (2021), "Crowdsourcing biocuration: the community assessment of community annotation with ontologies (cacao)." *PLoS computational biology*, 17, e1009463.

Ramsey, Jolene, Helena Rasche, Cory Maughmer, Anthony Criscione, Eleni Mijalis, Mei Liu, James C Hu, Ry Young, and Jason J Gill (2020), "Galaxy and apollo as a biologist-friendly interface for high-quality cooperative phage genome annotation." *PLOS Computational Biology*, 16, e1008214.

Rödelsperger, Christian, Marina Athanasouli, Maša Lenuzzi, Tobias Theska, Shuai Sun, Mohannad Dardiry, Sara Wighard, Wen Hu, Devansh Raj Sharma, and Ziduan Han (2019), "Crowdsourcing and the feasibility of manual gene annotation: a pilot study in the nematode pristionchus pacificus." *Scientific Reports*, 9, 18789.

Rutherford, Kim, Julian Parkhill, James Crook, Terry Horsnell, Peter Rice, Marie-Adèle Rajandream, and Bart Barrell (2000), "Artemis: sequence visualization and annotation." *Bioinformatics*, 16, 944–945.

Rutherford, Kim M, Midori A Harris, Antonia Lock, Stephen G Oliver, and Valerie Wood (2014), "Canto: an online tool for community literature curation." *Bioinformatics*, 30, 1791–1792.

Salamov, Asaf A and Victor V Solovyev (2000), "Ab initio gene finding in drosophila genomic dna." *Genome research*, 10, 516–522.

Salisbury, Alicia and Philippos K Tsourkas (2019), "A method for improving the accuracy and efficiency of bacteriophage genome annotation." *International journal of molecular sciences*, 20, 3391.

Sapoval, Nicolae, Amirali Aghazadeh, Michael G Nute, Dinler A Antunes, Advait Balaji, Richard Baraniuk, CJ Barberan, Ruth Dannenfelser, Chen Dun, Mohammadamin Edrisi, et al. (2022), "Current progress and open challenges for applying deep learning across the biosciences." *Nature Communications*, 13, 1728.

Sayers, Eric W, Mark Cavanaugh, Karen Clark, James Ostell, Kim D Pruitt, and Ilene Karsch-Mizrachi (2020), "Genbank." *Nucleic acids research*, 48, D84–D86.

Scalzitti, Nicolas, Anne Jeannin-Girardon, Pierre Collet, Olivier Poch, and Julie D Thompson (2020), "A benchmark study of ab initio gene prediction methods in diverse eukaryotic organisms." *BMC genomics*, 21, 1–20.

Schnoes, Alexandra M, Shoshana D Brown, Igor Dodevski, and Patricia C Babbitt (2009), "Annotation error in public databases: misannotation of molecular function in enzyme superfamilies." *PLoS computational biology*, 5, e1000605.

Schoonderwoerd, Tjeerd AJ, Emma M Van Zoelen, Karel van den Bosch, and Mark A Neerincx (2022), "Design patterns for human-ai co-learning: A wizard-of-oz evaluation in an urban-search-and-rescue task." *International Journal of Human-Computer Studies*, 164, 102831.

Shipley, Bill (2016), *Cause and correlation in biology: a user's guide to path analysis, structural equations and causal inference with R*. Cambridge university press.

Solovyev, Victor, Peter Kosarev, Igor Seledsov, and Denis Vorobyev (2006), "Automatic annotation of eukaryotic genes, pseudogenes and promoters." *Genome biology*, 7, 1–12.

Stanke, Mario, Oliver Keller, Irfan Gunduz, Alec Hayes, Stephan Waack, and Burkhard Morgenstern (2006), "Augustus: ab initio prediction of alternative transcripts." *Nucleic acids research*, 34, W435–W439.

Stanke, Mario, Stephan Waack, et al. (2003), "Gene prediction with a hidden markov model and a new intron submodel." *Bioinformatics-Oxford*, 19, 215–225.

Stein, Lincoln (2001), "Genome annotation: from sequence to biology." *Nature reviews genetics*, 2, 493–503.

Talukder, Amlan, Clayton Barham, Xiaoman Li, and Haiyan Hu (2021), "Interpretation of deep learning in genomics and epigenomics." *Briefings in Bioinformatics*, 22, bbaa177.

Tchechmedjiev, Andon, Amine Abdaoui, Vincent Emonet, Soumia Melzi, Jitendra Jonnagaddala, and Clement Jonquet (2018), "Enhanced functionalities for annotating and indexing clinical text with the ncbo annotator+." *Bioinformatics*, 34, 1962–1965.

Tello-Ruiz, Marcela K, Cristina F Marco, Fei-Man Hsu, Rajdeep S Khangura, Pengfei Qiao, Sirjan Sapkota, Michelle C Stitzer, Rachael Wasikowski, Hao Wu, Junpeng Zhan, et al. (2019), "Double triage to identify poorly annotated genes in maize: The missing link in community curation." *PLoS One*, 14, e0224086.

The UniProt Consortium (2023), "Uniprot: the universal protein knowledgebase in 2023." *Nucleic Acids Research*, 51, D523–D531.

Tiwari, Shrish, S Ramachandran, Alok Bhattacharya, Sudha Bhattacharya, and Ramakrishna Ramaswamy (1997), "Prediction of probable genes by fourier analysis of genomic sequences." *Bioinformatics*, 13, 263–270.

Vallenet, David, Laurent Labarre, Zoe Rouy, Valerie Barbe, Stephanie Bocs, Stephane Cruveiller, Aurelie Lajus, Geraldine Pascal, Claude Scarpelli, and Claudine Medigue (2006), "Mage: a microbial genome annotation system supported by synteny results." *Nucleic acids research*, 34, 53–65.

van Baren, Marijke J and Michael R Brent (2006), "Iterative gene prediction and pseudogene removal improves genome annotation." *Genome research*, 16, 678–685.

van den Bosch, Karel, Tjeerd Schoonderwoerd, Romy Blankendaal, and Mark Neerincx (2019), "Six challenges for human-ai co-learning." In *Adaptive Instructional Systems: First International Conference, AIS 2019, Held as Part of the 21st HCI International Conference, HCII 2019, Orlando, FL, USA, July 26–31, 2019, Proceedings 21*, 572–589, Springer.

van der Wal, Douwe, Iny Jhun, Israa Laklouk, Jeff Nirschl, Lara Richer, Rebecca Rojansky, Talent Theparee, Joshua Wheeler, Jörg Sander, Felix Feng, et al. (2021), "Biological data annotation via a human-augmenting ai-based labeling system." *NPJ Digital Medicine*, 4, 145.

Wang, Zifeng, Zizhao Zhang, Chen-Yu Lee, Han Zhang, Ruoxi Sun, Xiaoqi Ren, Guolong Su, Vincent Perot, Jennifer Dy, and Tomas Pfister (2022), "Learning to prompt for continual learning." In *Proceedings of the IEEE/CVF conference on computer vision and pattern recognition*, 139–149.

Watson, Joseph L, David Juergens, Nathaniel R Bennett, Brian L Trippe, Jason Yim, Helen E Eisenach, Woody Ahern, Andrew J Borst, Robert J Ragotte, Lukas F Milles, et al. (2023), "De novo design of protein structure and function with rfdiffusion." *Nature*, 620, 1089–1100.

Wei, Chih-Hsuan, Alexis Allot, Robert Leaman, and Zhiyong Lu (2019), "Pubtator central: automated concept annotation for biomedical full text articles." *Nucleic acids research*, 47, W587–W593.

Wilkerson, Matthew D, Shannon D Schlueter, and Volker Brendel (2006), "yrgate: a web-based gene-structure annotation tool for the identification and dissemination of eukaryotic genes." *Genome Biology*, 7, 1–11.

Yoo, Danny, Iris Xu, Tanya Z Berardini, Seung Yon Rhee, Vijay Narayanasamy, and Simon Twigger (2006), "Pubsearch and pubfetch: a simple management system for semiautomated retrieval and annotation of biological information from the literature." *Current Protocols in Bioinformatics*, 13, 9–7.

Zhang, Qiang, Keyang Ding, Tianwen Lyv, Xinda Wang, Qingyu Yin, Yiwen Zhang, Jing Yu, Yuhao Wang, Xiaotong Li, Zhuoyi Xiang, et al. (2024), "Scientific large language models: A survey on biological & chemical domains." *arXiv preprint arXiv:2401.14656.*

Zheng, Nan-ning, Zi-yi Liu, Peng-ju Ren, Yong-qiang Ma, Shi-tao Chen, Si-yu Yu, Jian-ru Xue, Ba-dong Chen, and Fei-yue Wang (2017), "Hybrid-augmented intelligence: collaboration and cognition." *Frontiers of Information Technology & Electronic Engineering*, 18, 153–179.

Zhou, Zhongliang, Mengxuan Hu, Mariah Salcedo, Nathan Gravel, Wayland Yeung, Aarya Venkat, Dongliang Guo, Jielu Zhang, Natarajan Kannan, and Sheng Li (2023), "Xai meets biology: A comprehensive review of explainable ai in bioinformatics applications." *arXiv preprint arXiv:2312.06082.*

Zou, James, Mikael Huss, Abubakar Abid, Pejman Mohammadi, Ali Torkamani, and Amalio Telenti (2019), "A primer on deep learning in genomics." *Nature genetics*, 51, 12–18.
